# Supplementary material for: Impact of Community Structure on Cascades
Source: arXiv:1606.00858 source file (2022-05-04)
Supplement: Supplementary file 1 [file highprobevent.tex]

{\color{red}The proof follows by Lemma~\ref{lem:initcond_conv} and the fact that the initial conditions \eqref{eq:ode_ic} appear as coefficient in the definition of $\Ffuncbold$. The idea is to construct a set $\widetilde{\mathcal{E}}(n,\kappa,\rho_0)\subset\mathcal{E}(n,\kappa)$ for a small enough constant $\rho_0>0$ such that $\lim_{n\to\infty}\prob(\widetilde{\mathcal{E}}(n,\kappa,\rho_0)) = 1$.
Let $\widetilde{\mathcal{E}}(n,\kappa,\rho_0)$ denote the set of initial conditions~\eqref{eq:ode_ic} that satisfies the following inequalities, for all $j\in\{1,2\}$, $d_j,d_{-j}\in\mathbb{Z}_+$, and $d_j+d_{-j}\leq d_{\max}$:
\begin{align*}
	&\abs{i^{(j)}_{d_j,d_{-j},0,0}(0)\,d_j/\lambda_j - \prob_{j*,m}(d_j,d_{-j})(1-\alpha_j(d_j,d_{-j}))} < \rho, \allowdisplaybreaks\\ &\abs{i^{(-j)}_{d_{-j},d_{j},0,0}(0)\,d_j/\lambda_m - \prob_{-j,m*}(d_{-j},d_{j})(1-\alpha_{-j}(d_{-j},d_{j}))} < \rho,\allowdisplaybreaks\\
	&\abs{w_j(0)/\lambda_j - \sum_{d_j+d_{-j} > d_{\max}}\prob_{j*,m}(d_j,d_{-j})(1-\alpha_j(d_j,d_{-j}))} < \rho,\allowdisplaybreaks\\
	&\abs{w^{(-j)}_m(0)/\lambda_m - \sum_{d_j+d_{-j} > d_{\max}}\prob_{-j,m*}(d_{-j},d_{j})(1-\alpha_{-j}(d_{-j},d_{j}))} < \rho.
\end{align*}
By Lemma~\ref{lem:initcond_conv}, for any constant $\rho>0$, we have $\lim_{n\to\infty}\prob(\widetilde{\mathcal{E}}(n,\kappa,\rho)) = 1$.

Let $k_0\in \mathbb{N}$ to be large enough such that $\norm{\Ffuncbold_{\infty}^{k_0}(\bs{1}) - \bs{\mu}_{*,\infty}}_\infty < \kappa^2/8$ which exists due to Corollary \ref{cor:Fprop_sol}. Let $\epsilon_1 = \inf\{\norm{\left(\bs{\mu} - \Ffuncbold_{\infty}(\bs{\mu})\right)_-}_\infty: \norm{\bs{\mu} - \bs{\mu}_{*,\infty}}_{\infty} =  \kappa^2/4 \text{ and }\bs{\mu} \ngtr \bs{\mu}_{*,\infty}\}$, and $\epsilon_2 = \inf\{\norm{\left(\bs{\mu} - \Ffuncbold_{\infty}(\bs{\mu})\right)_-}_\infty: \norm{\bs{\mu} - \bs{\mu}_{*,\infty}}_\infty =  \kappa \text{ and }\bs{\mu} \ngtr \bs{\mu}_{*,\infty}\}$ where for a vector $\bs{x} = (x_1,x_2,x_3,x_4)$ we define $(\bs{x})_- \coloneqq (x_1',x_2',x_3',x_4')$ such that $x_i' = x_i$ if $x_i<0$ and $x_i'=0$ otherwise. Note that $\epsilon_1,\epsilon_2 > 0$, since $\bs{\mu}_{*,\infty}$ is stable.

Let $\rho_1>0$ to be small enough, independent of $n$, such that for any initial condition~\eqref{eq:ode_ic} in $\widetilde{\mathcal{E}}(n,\kappa,\rho_1)$ the followings hold:
\begin{align*}
	&(a)~\norm{\Ffuncbold_{\infty}^{k_0}(\bs{1}) - \Ffuncbold^{k_0}(\bs{1})}_\infty < \kappa^2/8,\\
	&(b)~\sup\{\norm{\Ffuncbold(\bs{\mu}) - \Ffuncbold_{\infty}(\bs{\mu})}_\infty: \norm{\bs{\mu} - \bs{\mu}_{*,\infty}}_{\infty} =  \kappa^2/4  \text{ and }\bs{\mu} \ngtr \bs{\mu}_{*,\infty}\} < \epsilon_1/2,\\
	&(c)~\sup\{\norm{\Ffuncbold(\bs{\mu}) - \Ffuncbold_{\infty}(\bs{\mu})}_\infty: \norm{\bs{\mu} - \bs{\mu}_{*,\infty}}_{\infty} =  \kappa \text{ and }\bs{\mu} \ngtr \bs{\mu}_{*,\infty}\} < \epsilon_2/2,
\end{align*}
Note that $\Ffuncbold^{k_0}(\bs{1})$ is a continuous function of the initial conditions \eqref{eq:ode_ic}. 

The choice of $k_0$ together with $(a)$ implies that $\norm{\Ffuncbold^{k_0}(\bs{1}) - \bs{\mu}_{*,\infty}}_{\infty} <  \kappa^2/4$. Moreover, stability of $\bs{\mu}_{*,\infty}$ together with $(b)$ implies that $\Ffuncbold(\bs{\mu}) \nleq \bs{\mu}$, for all $\bs{\mu} \ngtr \bs{\mu}_{*,\infty} \text{ with }\norm{\bs{\mu} - \bs{\mu}_{*,\infty}}_{\infty} =  \kappa^2/4$. Combining these with Lemma \ref{lem:Fprop_feasreg}, we have $\norm{\bs{\mu}_{*} - \bs{\mu}_{*,\infty}}_{\infty} <  \kappa^2/2$. It is also easy to see that $(c)$ together with the choice of $\epsilon_2$ implies that $\Ffuncbold(\bs{\mu}) \nleq \bs{\mu}$, for all $\bs{\mu} \ngtr \bs{\mu}_{*,\infty} \text{ with } \norm{\bs{\mu} - \bs{\mu}_{*,\infty}}_\infty = \kappa$.

Next, let $\rho_2 < \rho_1$ to be small enough such that 
\begin{align*}
	&(d)~\left(\{\bs{\mu}: \mu_{j,j'} < 2\kappa\sqrt{\lambda_{\min}} \text{ for some }j\in\{1,2\}\} \setminus \mathcal{B}\left(\bs{\mu}_{*},\kappa^2\right)\right) \cap \mathcal{U} = \emptyset \text{  and  }\\
	&(e)~\forall \bs{\mu} \ngtr \bs{\mu}_{*,\infty} \text{ with } \norm{\bs{\mu} - \bs{\mu}_{*,\infty}}_\infty = \kappa: \text{ there exists $j\in\{1,2\}$ such that either}\\
	&\myquad[6]\frac{\mu^{(j,j)}_{*} -\kappa}{\mu^{(j,j)}_{*}} \Ffunc_{(j,j)}(\mu^{(j,j)},\mu^{(j,-j)}) > \mu^{(j,j)} 
	\text{  or  }\\
	&\myquad[6]\frac{\mu^{(1,2)}_{*}\mu^{(2,1)}_{*} - \kappa}{\mu^{(1,2)}_{*}\mu^{(2,1)}_{*}}\Ffunc_{(j,-j)}(\mu^{(-j,-j)},\mu^{(-j,j)}) > \mu^{(j,-j)}.
\end{align*}
Existence of $\rho_2$ follows by the similar logic and the fact that $\kappa< \kappa_1 < \kappa_0$.

Finally, note that the if $\rho < \rho_2$ is small enough, then the trajectory of ODEs with initial condition~\eqref{eq:ode_ic} in $\widetilde{\mathcal{E}}(n,\kappa,\rho)$ stays arbitrary close to the trajectory of $\bs{\mu}_\infty(t)$, before either of them to get settled at its equilibrium point. In particular, since
\begin{align*}
	\{\bs{\mu}_\infty(t) \text{ for }t\geq 0\} \setminus \mathcal{B}\left(\bs{\mu}_{*,\infty},\kappa^2/2\right)  \subset \mathcal{D}_{2\varepsilon(\kappa),\infty}
\end{align*}
and $\norm{\bs{\mu}_{*} - \bs{\mu}_{*,\infty}}_{\infty} <  \kappa^2/4$, we can pick $0<\rho_0<\rho_2$ so that
\begin{align*}
	\{\bs{\mu}(t) \text{ for }t\geq0\} \setminus \mathcal{B}\left(\bs{\mu}_{*},\kappa^2\right)  \subset \mathcal{D}_{\varepsilon(\kappa)},
\end{align*}
for ODEs with initial condition~\eqref{eq:ode_ic} in $\widetilde{\mathcal{E}}(n,\kappa,\rho_0)$.
}
