# Supplementary material for: Impact of Community Structure on Cascades
Source: arXiv:1606.00858 source file (2022-05-04)
Supplement: Supplementary file 2 [file odesmaininf.tex]

Throughout the proof, we use the subscript $n$ to denote the case of finite $n$ (total number of vertices), and we use no subscript to denote the behavior as $n\to\infty$, i.e., when we use the right-hand side of \eqref{eq:asyminitval} as initial condition rather than the actual initial condition \eqref{eq:ode_ic} given in Appendix \ref{app:odederive} (which is random). The proof is done via two steps: first, we analyze the case when $d_{\max} < \infty$; next, we relax this restriction for part \ref{thm:odesmaininf_2} of Theorem \ref{thm:odesmaininf}. Note that we use the function $\bs{F} = (F_{(1,1)},F_{(1,2)},F_{(2,1)},F_{(2,2)})$ given by \eqref{eq:trunc_Fjj}-\eqref{eq:trunc_Fj-j} which is the same as the function $\bs{F}$ given by the right-hand side of \eqref{eq:meanfield_mujj}-\eqref{eq:meanfield_muj-j}, if we use the right-hand side of \eqref{eq:asyminitval} as the initial condition.

Before proceeding with the discussion of these two steps, we present four preliminary lemmas that is used in the proof. The first lemma concerns with fixed points on the axis of origin. The other 3 lemmas relates the trajectory of $\bs{\mu}_n(t)$ to the trajectory of $\bs{\mu}(t)$, where $\bs{\mu}_n(t)$ and $\bs{\mu}(t)$ are the solutions of the ODE \eqref{eq:alterode} with functions $\bs{F}_n$ and $\bs{F}$ respectively.

\begin{lemma}\label{lem:zerosol}
	Let $\bs{\mu}_{*}\coloneqq\lim_{s\to\infty}\bs{F}^s(\bs{\bs{1}})$ to be the closest fixed point of $\bs{F}$ to $\bs{1}$ in sup norm. Assume at least one of the components of $\bs{\mu}_{*}$ is zero. Then, we have $\bs{\mu}_{*} = \bs{0}$.
\end{lemma}
\begin{proof}[proof of Lemma]
	The proof is similar to the proof of Lemma \ref{lem:Fprop_feasreg} part \ref{lem:Fprop_feasreg_iv}. Without loos of generality, assume $\mu_{*}^{(1,1)} = 0$. Since $\bs{F}$ is a non-negative function, using Lemma \ref{lem:Fprop_increasing}, we have $\mu_{*}^{(1,2)} = 0$ as $\bs{0} \leq \bs{\mu}_{*}$. Using the exact same argument, we have $\mu_{*}^{(2,2)} = \mu_{*}^{(2,1)} = 0$.
\end{proof}

\begin{lemma}\label{lem:stableregion}
	Let $\bs{\mu}_{*}\coloneqq\lim_{s\to\infty}\bs{F}^s(\bs{\bs{1}})$ to be the closest fixed point of $\bs{F}$ to $\bs{1}$ in sup norm. Assume $\bs{\mu}_{*}$ is an stable equilibrium of ODE \eqref{eq:alterode}, and assume $\bs{\mu}_{*} > \bs{0}$ component-wise. For any $\upsilon > 0$, define the set $\mathcal{A}_{\upsilon}$ as follows:
	\begin{align*}
	\mathcal{A}_{\upsilon} \coloneqq \left(\mathcal{B}(\bs{\mu}_{*},\upsilon) \cup \mathcal{A}\right) \setminus \text{int}(\mathcal{B}(\bs{\mu}_{*},\upsilon) )
	\end{align*}
	where $\mathcal{A}$ is given by \eqref{eq:setA}, $\mathcal{B}(\bs{x},\upsilon)$ is a ball of radius $\upsilon$ centered at $\bs{x}$, and $\text{int}(\mathcal{C})$ is the interior of the set $\mathcal{C}$. The $2$-dimensional schematic of $\mathcal{A}_\upsilon$ is given in Figure~\ref{fig:schematicAups}.
	\begin{figure}[t!]
		\centering
		\includegraphics[width=0.5\textwidth]{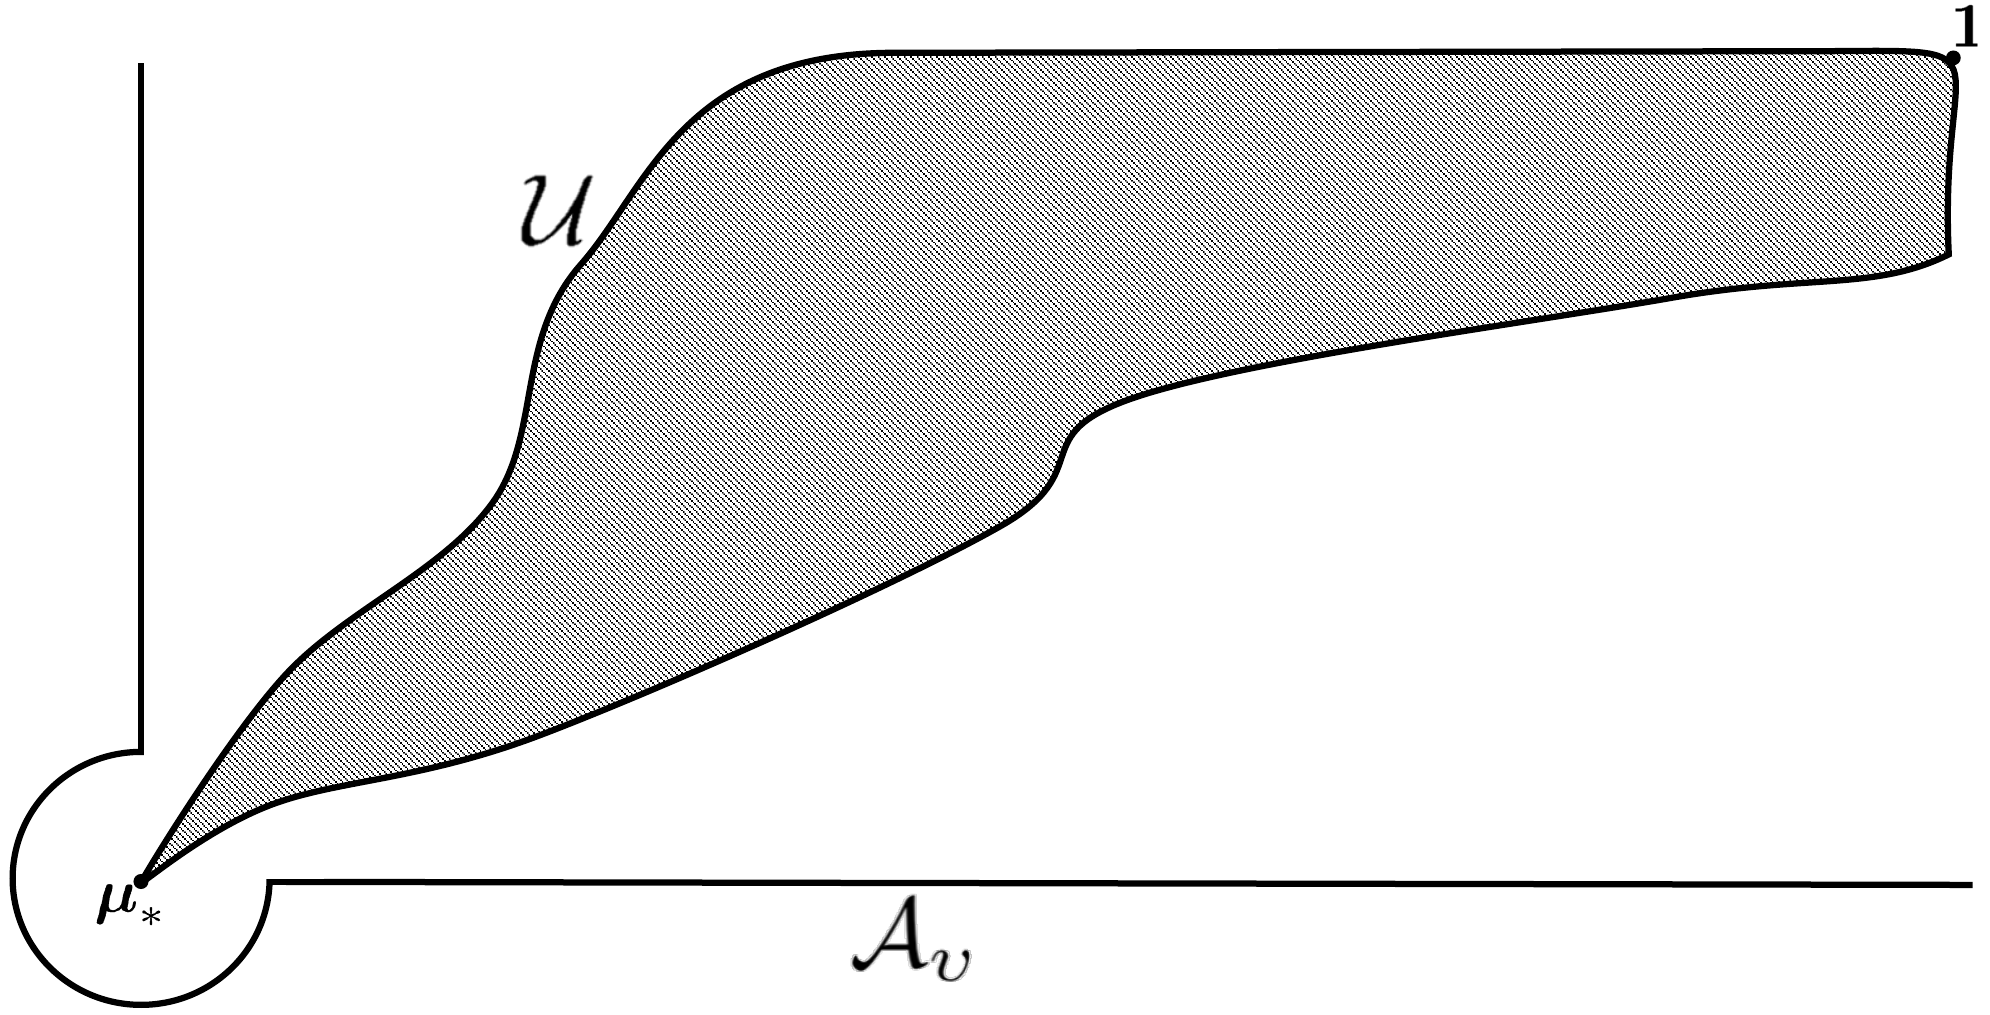}
		\caption{Schematic of $\mathcal{A}_{\upsilon}$.}\label{fig:schematicAups}
	\end{figure}
	Then, there is a small enough $\upsilon_0 > 0$ such that $\mathcal{A}_{\upsilon_0} \subset (0,1]^4$ and $\bs{F}(\bs{u}) \nleq \bs{u}$ component-wise,  $\forall \bs{u}\in\mathcal{A}_{\upsilon_0}$. Moreover, we have $\bs{F}_n(\bs{u}) \nleq \bs{u}$ with high probability; that is to say, for any $p > 0$ there is a large enough $n_p > 0$ such that for any $n > n_p$, the event $\{\bs{F}_n(\bs{u}) \nleq \bs{u},~\forall \bs{u}\in\mathcal{A}_{\upsilon_0}\}$ holds with probability greater than $1-p$. 
\end{lemma}
\begin{proof}[proof of Lemma]
	By part \ref{lem:Fprop_feasreg_iv} of Lemma \ref{lem:Fprop_feasreg}, for all $\bs{u} \in \mathcal{A}$ we have ${\bs{F}}(\bs{u}) \nleq \bs{u}$. Since $\bs{\mu}_{*}$ is an stable equilibrium point, $\exists \upsilon_1 > 0$ such that starting from any point $\bs{u} \in \mathcal{B}(\bs{\mu}_{*},\upsilon_1)\subset (0,1]^4$, the ODE \eqref{eq:alterode} converges to $\bs{\mu}_{*}$. Next, we show that if ${\bs{F}}(\bs{u}) \leq \bs{u}$ for some $\bs{u} \in \mathcal{B}(\bs{\mu}_{*},\upsilon_1)$, then $\bs{u} \geq \bs{\mu}_{*}$ component-wise.
	
	By the same argument as in the proof of Theorem \ref{thm:alterode_sol}, if ${\bs{F}}(\bs{u}) \leq \bs{u}$ then the ODE \eqref{eq:alterode} starting from $\bs{u}$ converges to the fixed point $\lim_{s\to\infty}\bs{F}^s(\bs{u})$ which is smaller than $\bs{u}$ component-wise. Hence, $\bs{u} \geq \bs{\mu}_{*}$ so that $\bs{\mu}_{*}=\lim_{s\to\infty}\bs{F}^s(\bs{u})$.
	
	Let $\upsilon_0 = \upsilon_1/2$. By the above argument, we have $\bs{F}(\bs{u}) \nleq \bs{u}$ component-wise,  $\forall \bs{u}\in\mathcal{A}_{\upsilon_0}$. Pick $\varepsilon_0 > 0$ small enough such that $\bs{F}(\bs{u}) - \varepsilon_0\bs{1} \nleq \bs{u}$ for all $\bs{u} \in \mathcal{A}_{\upsilon_0}$. Now, using \eqref{eq:asyminitval} and the fact that the dependency of $\bs{F}$ to the initial condition is through coefficients, for any $p>0$ we can pick $n_p > 0$ large enough such that for any fixed $n>n_p$ the event $\{\forall \bs{u}\in\mathcal{A}_{\upsilon_0}: \norm{\bs{F}(\bs{u}) - \bs{F}_n(\bs{u})}_\infty < \varepsilon_0/2\}$ holds with probability greater than $1-p$. 
\end{proof}
\begin{lemma}\label{lem:stablesol}
	Let $\bs{\mu}_{*}\coloneqq\lim_{s\to\infty}\bs{F}^s(\bs{\bs{1}})$ and $\bs{\mu}_{*,n}\coloneqq\lim_{s\to\infty}\bs{F}^s_n(\bs{\bs{1}})$ to be the closest fixed point of $\bs{F}$ and $\bs{F}_n$ to $\bs{1}$ in sup norm, receptively. Note that $\bs{\mu}_{*,n}$ is a random variable as it depends on the initialization. Assume $\bs{\mu}_{*}$ is an stable equilibrium of ODE \eqref{eq:alterode}. Then, for any $\zeta>0$,  $\bs{\mu}_{*,n} \in \mathcal{B}(\bs{\mu}_{*},2\zeta)$, with high probability.
\end{lemma}
\begin{proof}[proof of Lemma]
	Pick $k$ large enough such that $\bs{F}^k(\bs{\bs{1}}) \in \mathcal{B}(\bs{\mu}_{*},\zeta)$. Now, using \eqref{eq:asyminitval}, we have $\bs{F}^k_n(\bs{\bs{1}}) \in \mathcal{B}(\bs{\mu}_{*},2\zeta)$ with high probability. If $\bs{\mu}_{*} = \bs{0}$, the proof is complete. Otherwise, by Lemma \ref{lem:zerosol}, we have $\bs{\mu}_{*} > 0$ component-wise. In the later case, using Lemma \ref{lem:stableregion}, for small enough $\upsilon_0 < 2\zeta$, we have $\mathcal{A}_{\upsilon_0} \cap \mathcal{U}_n = \emptyset$ with high probability (Recall that $\mathcal{U}_n$ is the largest connected set containing $\bs{1}\coloneqq(1,1,1,1)$ such that $\forall \bs{u}\in \mathcal{U}$, $\bs{u} \geq \bs{F}_n(\bs{u})$. ).  Hence, $\lim_{s\to\infty}\bs{F}^s_n(\bs{\bs{1}}) \in \mathcal{B}(\bs{\mu}_{*},2\zeta)$ with high probability.
\end{proof}

\noindent\textbf{Step 1:} Assume there is a constant $\infty > d_{\max} > 0$ such that for all $d_j+d_{-j} > d_{\max}$, we have $K_j(d_j,d_{-j}) = d_j+d_{-j}$; that is to say, the inactive vertices with degree higher than $d_{\max}$ cannot be activated.

Now, the proof of part \ref{thm:odesmaininf_1} of Theorem \ref{thm:odesmaininf} follows immediately from Theorem \ref{thm:odesfinite}, Lemma \ref{lem:diffeq_sol}, and the fact that the trajectory of $\bs{\mu}_{n}(x)$ and $\bs{\mu}(x)$ are uniformly close to each other with high probability. The last statement follows by the exact same argument as in the proof of Lemma \ref{lem:stableregion}: for any $\varepsilon_0 > 0$, we can pick $n_p > 0$ large enough such that the probability of the event $\{\forall \bs{u} \geq \bs{\mu}_{t}: \norm{\bs{F}(\bs{u}) - \bs{F}_n(\bs{u})}_\infty < \varepsilon_0\}$ is less than $1-p$ for all $n>n_p$. %Recall that $t<t_*$ corresponds to some point $\bs{\mu}_{t} > \bs{0}$ which is strictly greater than $\bs{\mu}_{*}$ component-wise. Also note that $$\frac{d\bs{\mu}_n}{dt} = \frac{d\bs{\mu}}{dt} + \bs{F}_n(\bs{u}) - \bs{F}(\bs{u}).$$

For the proof of part \ref{thm:odesmaininf_2} of Theorem \ref{thm:odesmaininf}, we use the idea that we introduced in Section \ref{sec:odeanalysisinf}. We skip some minor details, as we have already used similar arguments in other parts of the paper. If $\bs{\mu}_* = \bs{0}$ there is nothing to prove as all the half-edges has been used and the process has to stop. Note that by Lemma \ref{lem:stablesol}, $\bs{\mu}_{*,n}$ is in any fixed ball around $\bs{\mu}_*$ with high probability.

Now, assume $\bs{\mu}_* \neq \bs{0}$. By Lemma \ref{lem:zerosol}, we know $\bs{\mu}_* >\bs{0}$ component-wise. By Lemma \ref{lem:stableregion}, we can pick $\upsilon_0 > 0$ small enough such that $\mathcal{A}_{\upsilon_0} \cap \mathcal{U} = \emptyset$ and for all $\bs{u}\in\mathcal{A}_{\upsilon_0}$ we have $\bs{u} > 0$ component-wise. Following the proof of Lemma \ref{lem:stableregion}, let $\varepsilon_0>0$ to be small enough such that $\bs{F}(\bs{u}) - \varepsilon_0\bs{1} \nleq \bs{u}$ for all $\bs{u} \in \mathcal{A}_{\upsilon_0}$. Note that the event $\{\forall \bs{u}\in\mathcal{A}_{\upsilon_0}: \norm{\bs{F}(\bs{u}) - \bs{F}_n(\bs{u})}_\infty < \varepsilon_0/2\}$ holds with high probability. Define $\bs{F}_{n,\kappa}(\bs{u})$ as in \eqref{eq:trunc_Fjj}-\eqref{eq:trunc_Fj-j} by replacing the the terms $\lambda_1$, $\lambda_2$, and $\lambda_m$ with $\lambda_1 + \kappa$, $\lambda_2 + \kappa$, and $\lambda_m + \kappa$. Let $\kappa_0>0$ to be small enough such that $\{\forall \bs{u}\in\mathcal{A}_{\upsilon_0}: \norm{\bs{F}_{n,\kappa_0}(\bs{u}) - \bs{F}_n(\bs{u})}_\infty < \varepsilon_0/4\}$ holds with high probability. Also, note that by Lemma \ref{lem:stablesol}, we have $\bs{\mu}_{*,n} \in \mathcal{B}(\bs{\mu}_{*},\upsilon_0/4)$ with high probability.

To summarize the crucial results so far, we have $\{\forall \bs{u}\in\mathcal{A}_{\upsilon_0}: \norm{\bs{F}_{n,\kappa_0}(\bs{u}) - \bs{F}(\bs{u})}_\infty < 3\varepsilon_0/4\}$ and $\bs{\mu}_{*,n} \in \mathcal{B}(\bs{\mu}_{*},\upsilon_0/4)$ with high probability, and $\bs{F}(\bs{u}) - \varepsilon_0\bs{1} \nleq \bs{u}$ for all $\bs{u} \in \mathcal{A}_{\upsilon_0}$. Recall the choice of $\gamma_0 > 0$ as in \eqref{eq:epschoice} (see Figure \ref{fig:schematic}). Consider a point $\bs{\mu}_{0,n} = \bs{\mu}_{n}(x_0) \in\mathcal{B}(\bs{\mu}_*,\gamma_0)$ on the trajectory of $\bs{\mu}_{n}$ such that
$
a_{1,n}(x_0) + a_{2,n}(x_0) + a_{m,n}^{(1)}(x_0) + a_{m,n}^{(2)}(x_0) = \kappa_0/2.
$
Note that such a point exists with high probability. At the corresponding time step of the process, the total number of active half-edges is of order of $\kappa_0 n$ with high probability, and we expect the Markov process of adoption stop shortly thereafter. 

At this point, we modify the process by adding one active vertex to each community, each of which has $\kappa_0 n$ active half-edges for in community connections and $\kappa_0 n$ half-edges for out community connections. In terms of one step drifts, we can recycle the one-step drifts in Appendix \ref{app:onestepdrift} by replacing the terms $m_1(n)$, $m_2(n)$, and $m_m(n)$ with $m_1(n)+\kappa_0 n $, $m_2(n) + \kappa_0 n$, and $m_m(n) + \kappa_0 n$. Similarly, this modification reflects in ODE by replacing $\bs{F}_n$ with $\bs{F}_{n,\kappa_0}$. Let $\bs{\mu}_{*,n}^{\kappa_0}$ denote the equilibrium point after modification. Trivially, $\bs{\mu}_{*,n}^{\kappa_0} \leq \bs{\mu}_{*,n}$ as $\mathcal{U}_n\subset \mathcal{U}_n^{\kappa_0}$. Moreover, $\mathcal{A}_{\upsilon_0} \cap \mathcal{U}_n^{\kappa_0} = \emptyset$ with high probability as $\{\forall \bs{u}\in\mathcal{A}_{\upsilon_0}: \norm{\bs{F}_{n,\kappa_0}(\bs{u}) - \bs{F}(\bs{u})}_\infty < 3\varepsilon_0/4\}$ with high probability. Finally, since $\bs{\mu}_{*,n} \in \mathcal{B}(\bs{\mu}_{*},\upsilon_0/4)$ with high probability, we have $\bs{\mu}_{*,n}^{\kappa_0} \in \text{int}(\mathcal{B}(\bs{\mu}_*,\upsilon_0))$ with high probability as well.

Using the exact same techniques as in Theorem \ref{thm:odesfinite} and Lemma \ref{lem:diffeq_sol}, we can track the modified process using the modified ODE (with the new set of initial condition given by the final values of the original ODE at the point of modification) up to any neighborhood of $\bs{\mu}_{*,n}^{\kappa_0}$. In particular, we can track the modified process upto when 
$
a_{1,n}(x) + a_{2,n}(x) + a_{m,n}^{(1)}(x) + a_{m,n}^{(2)}(x) = \kappa_0/2
$
for the modified ODE. At the corresponding time step of the modified process, we have already used all the original active half-edges from the original process, and most of the active half-edges from the modified one. Hence, if we ignore the modification, the original process runs out of active half-edges. Note that since $\bs{\mu}_{*} > \bs{0}$, we can pick $\upsilon_0$ small enough such that most of the newly added active half-edges are used to be connected to inactive vertices, i.e., they are not wasted. Now, the result follows by adjusting the constant $\upsilon_0$ to be arbitrary small.

\noindent\textbf{Step 2:} Consider the truncated processes $X^n_{L,\delta}$ and $X^n_{U,\delta}$ defined in Point \ref{point:2} of Section \ref{sec:odeapprox}. Let $\bs{F}_{L,\delta}$ and $\bs{F}_{U,\delta}$ denote the functions correspond to these processes, with the coefficients given by the right-hand side of \eqref{eq:asyminitval}. Let $\bs{\mu}_{*,L,\delta}$ and $\bs{\mu}_{*,U,\delta}$ denote the closets fixed points of $\bs{F}_{L,\delta}$ and $\bs{F}_{U,\delta}$ to $\bs{1}$ in sup norm respectively.

First off, note that for any $\delta > 0$, we have $\bs{F}_{U,\delta}(\bs{u}) < \bs{F}(\bs{u}) <\bs{F}_{L,\delta}(\bs{u})$ for all $\bs{u}\in[0,1]^4$. Moreover, $\bs{F}_{L,\delta}(\bs{u}) - \bs{F}_{U,\delta}(\bs{u}) < 2\delta$. Now, if we pick $\delta >0$ small enough, the trajectory of the corresponding ODEs (given by the functions $\bs{F}_{L,\delta}$, $\bs{F}_{U,\delta}$, and $\bs{F}$) are uniformly close to each other. It is also easy to see that the corresponding equilibrium points are arbitrary close to each other by small choice of $\delta$, whenever $\bs{\mu}_*$ is stable. Moreover, if $\bs{\mu}_*$ is stable, so are $\bs{\mu}_{*,L,\delta}$ and $\bs{\mu}_{*,U,\delta}$ for all small enough $\delta > 0$.

Now, the proof of part \ref{thm:odesmaininf_2} of Theorem \ref{thm:odesmaininf} for the case $d_{\max} = \infty$ follows by the fact that for small $\delta>0$, both truncated processes $X^n_{U,\delta}$ and $X^n_{L,\delta}$ stops at points arbitrary close to $\bs{\mu}_*$ (as $\bs{\mu}_{*,U,\delta}$ and $\bs{\mu}_{*,U,\delta}$ are arbitrary close to $\bs{\mu}_*$).
