# Supplementary material for: Impact of Community Structure on Cascades
Source: arXiv:1606.00858 source file (2022-05-04)
Supplement: Supplementary file 3 [file couple.tex]

Recall that in the augmented process, we first pair all the augmented half-edges with randomly selected regular half-edges and then we proceed normally. However, in the twisted process, we pair half-edges in three phases. At first, we pair a random regular active half-edge with a randomly selected half-edge in the appropriate community. If the second half-edge is an augmented one, we pick another augmented half-edge in the same community as the initial active half-edge and pair it with a random regular half-edge. Next, after removing all the regular active half-edges, we pair all the remaining augmented half-edges (if any) with random regular half-edges. Finally, we pair all the remaining active half-edges with random half-edges. Also, recall that for any $k>0$, $\Gamma_j(k)$ (resp., $\Gamma_m^{(j)}(k)$) is the time step in the twisted process for which the number of pair of half-edges removed from community $j$ (resp., between the communities) is equal to $\widetilde{T}_j(k)$ (resp., $\widetilde{T}_m(k)$). Note that if such time step does not exist, we set $\Gamma_j(k) = \infty$ (resp., $\Gamma_m^{(j)}(k) = \infty$).

Note that up to time step $\floor{t_\kappa n}$, both the augmented process and the twisted process follow the same sample path. After adding the augmented half-edges, we assign labels to all the remaining half-edges. At the beginning of time step $\floor{t_\kappa n}+1$, the label of half-edges in both processes are the same. As we proceed with the coupling, we may swap the label of half-edges in the augmented process with each other. Given a realization of the sample path of the twisted process, we realize a sample path for the augmented process by the following coupling.

To keep track of the events in the coupling, we define new sets of (random) variables $\{k_{j,j'}\}_{j,j'\in\{1,2\}}\in\mathbb{N}^4$ and $\{b_{j,j'}\}_{j,j'\in\{1,2\}} \in \{0,1\}^4$. We initialize these variables to be $\floor{t_\kappa n}$ and $0$ respectively. Consider a typical time step $k$ of the augmented process. Without loss of generality, suppose that at time step $k$ of the augmented process we are going to pair a random active half-edge $\widetilde{a}$ (regular or augmented) in community $j$ with another half-edge in the same community. Based on $\widetilde{a}$, the state of the twisted process and the value of $k_{j,j}$ and $b_{j,j}$, we realize the second half-edge as follows:
\begin{enumerate}[label=Case $\arabic*$:]
	\item At time step $k_{j,j}$, the twisted process is in the first phase. In this case, we have the following sub-cases:
	\begin{enumerate}[label=Case $1.\arabic*$:]
		\item $\widetilde{a}$ is an augmented half-edge. Update $k_{j,j} = \Gamma_j(k)$. Suppose that at time step $k_{j,j}$ of the twisted process, we paired an active half-edge $\widehat{a}$ (regular or augmented) with a random half-edge $\widehat{b}$. Based on $\widehat{a}$ and $\widehat{b}$, we do one of the followings:
		\begin{enumerate}[label=--]
			\item If $\widehat{a}$ is an augmented half-edge in the twisted process, then pair $\widetilde{a}$ with $\widehat{b}$ in the augmented process. Swap the label of the half-edges $\widetilde{a}$ and $\widehat{a}$ in the augmented process.
			\item If $\widehat{a}$ is a regular half-edge in the twisted process and $\widehat{b} = \widetilde{a}$, then pair $\widetilde{a}$ with $\widehat{a}$ in the augmented process.
			\item If both $\widehat{a}$ and $\widehat{b}$ are regular half-edges in the twisted process, then pair $\widetilde{a}$ with $\widehat{b}$ in the augmented process. Swap the label of the half-edges $\widetilde{a}$ and $\widehat{a}$ in the augmented process.
		\end{enumerate}
		Note that during this sub-case, the label of vertices 
	
	\end{enumerate}
	\item At time step $k_{j,j}$, the twisted process is not in the first phase. In this case, we decouple the two process, i.e., we pair $\widetilde{a}$ with a random half-edge in community $j$. Recall that if $\widetilde{a}$ is an augmented half-edge, we can only pair it with regular half-edges.
\end{enumerate}

However, after adding the augmented half-edges, they may follow different sample paths. 

To construct the coupling, we label half-edges so that the label of half-edges in community $j$ (resp., between the two communities) of the augmented process at time step $k$ is same as the label of half-edges in community $j$ (resp., between the two communities) of the twisted process at time step $\Gamma_j(k)$ (resp., $\Gamma_m^{(j)}(k)$). We relabel the half-edges during the augmented process to make sure that this property holds at any time $k \geq 0$ for which $\Gamma_j(k) < \infty$ (resp., $\Gamma_m^{(j)}(k)< \infty$). Now, given a realization of the sample path of the twisted process, we realize a sample path for the augmented process by the following coupling.

Consider a typical time step $k$ of the augmented process. Without loss of generality, let us assume that at time step $k$, we are going to pair two half-edges in community $j$. Recall that, if $\Gamma_j(k) < \infty$, then the label of half-edges at time step $k$ in community $j$ of the augmented process is same as the label of half-edges at time step $\Gamma_j(k)$ in community $j$ of the twisted process. Suppose that at time step $\Gamma_j(k)$ (if $\Gamma_j(k) < \infty$) of the twisted process, we paired ac active half-edge $\widehat{a}$ (regular or augmented) with a random half-edge $\widehat{b}$. Also, suppose that at time step $k$ of the augmented process we are going to pair a random active half-edge $\widetilde{a}$ (regular or augmented) with another half-edge. Based on the value of $\Gamma_j(k)$, $\widehat{a}$, $\widehat{b}$ and/ $\widetilde{a}$, we realize the second half-edge and then relabel the half-edges as follows:
