# Supplementary material for: Impact of Community Structure on Cascades
Source: arXiv:1606.00858 source file (2022-05-04)
Supplement: Supplementary file 4 [file coupling.tex]

To couple these two processes with each other, we we invoke the function $\text{swap}(\cdot,\cdot)$ repeatedly, which takes labels of two half-edges and swap the second part of the labels while keeping the first part intact:

$\{\widetilde{B}^{(j)}_s\}_{s\geq 1}$ denote the sequence of half-edges that are removed in community $j\in\{1,2\}$ after time $\floor{t_\kappa n}$, and let

We couple this realization with a realization of the Phase \ref{def:twist_phase1} of the twisted process, i.e., whenever the twisted process moved to Phase \ref{def:twist_phase2} or Phase \ref{def:twist_phase3}, we proceed the realization of the twisted process independent of the augmented process. As a notational convention, we use ``$\,\,\widetilde{~}\,\,$'' and ``$\,\,\widehat{~}\,\,$'' to denote variables associated with the augmented and twisted processes respectively.

%In the following coupling, we use a random relabeling function $\Upsilon$ that takes two equisized sets of labels of half-edges and map them to each other uniformly at random, while keeping the labels in their intersection intact. See Figure \ref{fig:labelreassign} for an example.
%\begin{figure}
%	\centering
%	\includegraphics[width=0.65\textwidth]{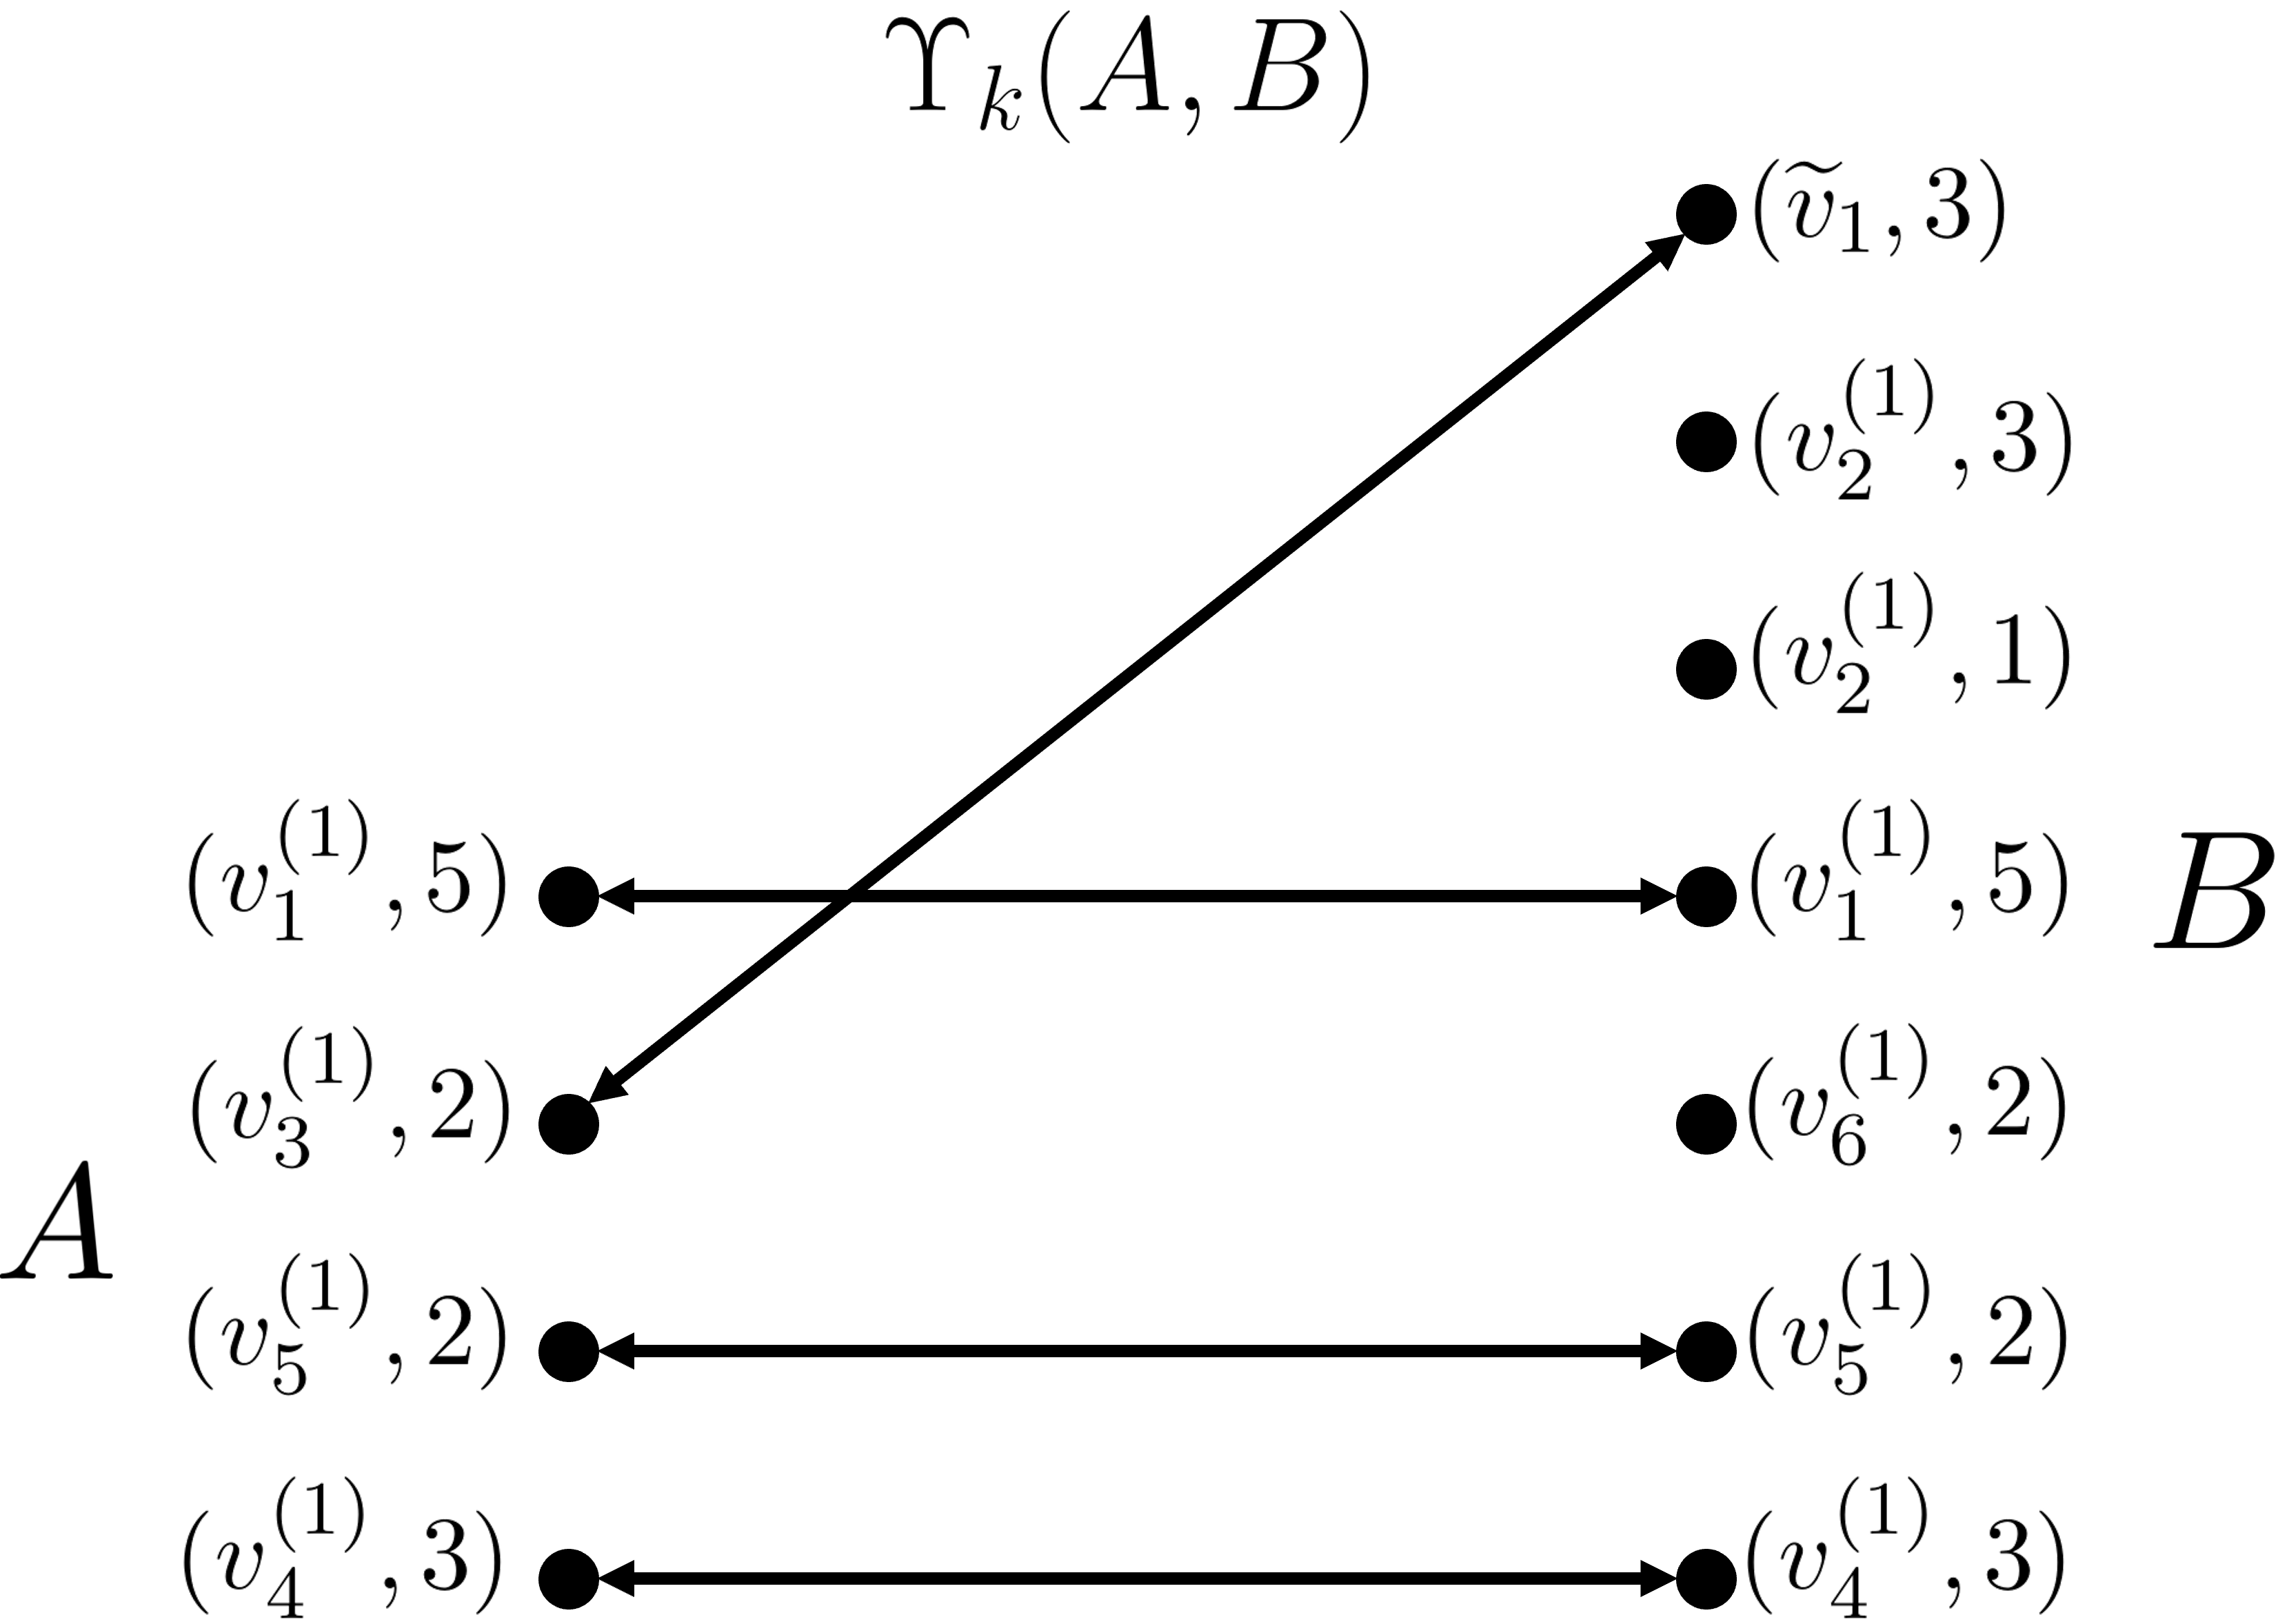}
%	\caption{A realization of the function $\Upsilon$ mapping the sets $\left\{(v_1^{(1)},1), (v_3^{(1)},4), (v_{10}^{(1)},2),(v_5^{(1)},4)\right\}$ and $\left\{ (v_3^{(1)},2), (v_2^{(1)},2), (v_1^{(1)},1),(v_3^{(1)},5)\right\}$ to each other. Note that their intersection $\left\{(v_1^{(1)},1)\right\}$ remains intact.
%	} \label{fig:labelreassign}
%\end{figure}

Consider a time $k > \floor{t_\kappa n}$ of the twisted process which corresponds to the beginning of an iteration in Phase \ref{def:twist_phase1}. Suppose that the label of the randomly selected regular active half-edge is $(\text{reg},(v_l^{(j)},i))$. Depending on the value of $i$, we have one of the following cases:
\begin{enumerate}[label=Case (\arabic*):]
	\item $i>0$.

	OK, in this case, you pick an active half-edge, keep removing half-edges till the outcome of a coin toss end up being like removing a regular half-edge, you look at the same state in the augmented process, apply the remapping function and then remove the corresponding half-edge. The point is that after removal of the half-edge, you have only remove half-edges in the twisted process that has already been removed in the augmented process.

	\item $i<0$. Pair with the same half-edge that it is going to be paired with after time RUNNING out of half-edges.
\end{enumerate}

 In the following coupling, we invoke the function $\text{swap}(\cdot,\cdot)$ repeatedly, which takes labels of an augmented half-edge and a regular half-edge and swap the second part of the labels while keeping the first part intact, e.g.,
\begin{align*}
	((\text{aug},(\widetilde{v}_j,i')),(\text{reg},(v_l^{(j)},i))) \xrightarrow{\text{swap}} ((\text{aug},(v_l^{(j)},i)),(\text{reg},(\widetilde{v}_j,i'))).
\end{align*}

\begin{enumerate}[label=Case (\arabic*):]
	\item $i>0$. Let $\widehat{T}_j^r(k)$ denote the number of iterations in which two regular half-edges are removed from community $j$ up to time $k$. Note that $\widehat{T}_j^r(k) \leq \widehat{T}_j(k)$. Depending on the value of $\widehat{T}_j^r(k)$, we have the following sub-cases:
	\begin{enumerate}[label=Sub-case (\roman*):]
		\item $\widehat{T}_j^r(k) > \floor{\kappa^{(j)} \lambda_j n/2}$. Consider the time at which we removed $\widehat{T}_j^r(k)+1$th pair of half-edges from community $j$ in the augmented process. Suppose that the label of the half-edges that are removed are $(\text{reg},(v_{l'}^{(j)},i'))$ and $(\text{reg},(v_{l''}^{(j)},i''))$ where $(\text{reg},(v_{l'}^{(j)},i'))$ is the active half-edge and $(\text{reg},(v_{l''}^{(j)},i''))$ is the random half-edge.

	\end{enumerate}
	 and $\widehat{T}(k) < \floor{\kappa^{(j)} \lambda_j n/2}$. Suppose that at time $\widetilde{T}(k)$
	\item $i<0$.
\end{enumerate}
