# Supplementary material for: Impact of Community Structure on Cascades
Source: arXiv:1606.00858 source file (2022-05-04)
Supplement: Supplementary file 5 [file additional_Note.tex]

For ease of explanation, we assume the same degree distribution for the cross-community links but we believe that our results hold even if this weren't the case.
